# Supplementary material for: Bootstrapping Non-Stationary Stochastic Volatility
Source: arXiv:2101.03562 ancillary file (2021-01-10)
Supplement: Supplementary file 1 [file BCGR_Appendix_2021_01_10_arXiv.pdf]

# BOOTSTRAPPING NON-STATIONARY STOCHASTIC VOLATILITY

H. PETER BOSWIJK<sup>a</sup>, GIUSEPPE CAVALIERE<sup>b,c</sup>, ILIYAN GEORGIEV<sup>b,d</sup>  
AND ANDERS RAHBEK<sup>e</sup>

## A ONLINE APPENDIX

### A.1 AUXILIARY RESULTS

Throughout, we make use of the following version of Skorokhod's representation theorem.

**THEOREM A.1** [*Kallenberg, 1997, Corollary 5.12*] *Let  $f$  and  $\{f_n\}_{n \geq 1}$  be measurable functions from a Borel space  $\mathcal{S}$  to a Polish space  $\mathcal{T}$ , and let  $\xi$  and  $\{\xi_n\}_{n \geq 1}$  be random elements in  $\mathcal{S}$  with  $f_n(\xi_n) \xrightarrow{w} f(\xi)$ . Then there exist some random elements  $\tilde{\xi} \stackrel{d}{=} \xi$  and  $\tilde{\xi}_n \stackrel{d}{=} \xi_n$  defined on a common probability space with  $f_n(\tilde{\xi}_n) \xrightarrow{a.s.} f(\tilde{\xi})$ .*

The next lemma contains a result about the asymptotic continuity of the distribution function of Dickey-Fuller type-statistics under non-stationary stochastic volatility.

**LEMMA A.1** *With  $M$  and  $V$  defined in Lemma 1, under Assumptions 1 and 2, let*

$$\tau_1 := \frac{\int_0^1 M(u) dM(u)}{\int_0^1 M^2(u) du} \quad \text{and} \quad \tau_2 := \frac{\int_0^1 M(u) dM(u)}{\sqrt{V(1) \int_0^1 M^2(u) du}}.$$

*Then the random cdfs  $F_1(\cdot) := P(\tau_1 \leq \cdot | \sigma)$  and  $F_2(\cdot) := P(\tau_2 \leq \cdot | \sigma)$  are sample-path continuous a.s.*

**PROOF OF LEMMA A.1.** We reduce the proof to the following well-known result (Rao and Swift, 2006, pp. 472–473). Let  $\{X(u)\}_{u \in [0,1]}$  be a Gaussian process with mean zero and a continuous covariance kernel, let  $q : [0, 1] \rightarrow \mathbb{R}$  be a square-integrable function and let  $\alpha \in \mathbb{R}$  be arbitrary. Then the distribution of  $\int_0^1 (X(u) + \alpha q(u))^2 du$  is that of an infinite series of independent non-central  $\chi^2$  random variables and, as a result, it has a continuous cdf.

The random cdfs  $F_1$  and  $F_2$  are determined, up to a modification, by the *distribution* of  $(B_z, \sigma)$ , such that the structure of the probability space on which  $(B_z, \sigma)$  is defined is irrelevant for the claim of interest. We therefore assume, without loss of generality, that the independent

---

<sup>a</sup>Amsterdam School of Economics and Tinbergen Institute, University of Amsterdam, The Netherlands

<sup>b</sup>Department of Economics, University of Bologna, Italy

<sup>c</sup>Department of Economics, Exeter Business School, UK

<sup>d</sup>Institut d'Anàlisi Econòmica (CSIC), Spain

<sup>e</sup>Department of Economics, University of Copenhagen, Denmark

Correspondence to: Giuseppe Cavaliere, Department of Economics, University of Bologna, Piazza Scaravilli 2, I-40126 Bologna, Italy. email: giuseppe.cavaliere@unibo.it.

processes  $B_z$  and  $\sigma$  are defined on a product probability space. Let  $(\Omega_\sigma, \mathcal{F}_\sigma, P_\sigma)$  be the factor-space on which  $\sigma$  is defined. Fix  $A \in \mathcal{F}_\sigma$  with  $P_\sigma(A) = 1$  such that  $V(\omega, \cdot) := \int_0^\cdot \sigma^2(\omega, u) du$  is well-defined, continuous and  $0 < V(\omega, 1) < \infty$ . Let  $\Gamma := \{\sigma(\omega, \cdot) : \omega \in A\}$  be the set of trajectories for  $\sigma$  when  $\omega \in A$ . For every  $\gamma \in \Gamma$ , the process  $M_\gamma(\cdot) := \int_0^\cdot \gamma(u) dB_z(u)$  is a.s. well-defined and  $\int_0^1 M_\gamma^2(u) du > 0$  a.s. The result in the lemma will follow if the deterministic cdfs  $P(\tau_{\gamma 1} \leq \cdot)$  and  $P(\tau_{\gamma 2} \leq \cdot)$  are continuous for every  $\gamma \in \Gamma$ :

$$P(\tau_{\gamma 1} = x) = 0, \quad P(\tau_{\gamma 2} = x) = 0, \quad \forall (x, \gamma) \in \mathbb{R} \times \Gamma, \quad (\text{A.1})$$

where

$$\tau_{\gamma 1} := \frac{\int_0^1 M_\gamma(u) dM_\gamma(u)}{\int_0^1 M_\gamma^2(u) du}, \quad \tau_{\gamma 2} := \frac{\int_0^1 M_\gamma(u) dM_\gamma(u)}{\sqrt{V(1) \int_0^1 M_\gamma^2(u) du}}.$$

In fact, (A.1) implies that  $F_1$  and  $F_2$  have sample-path continuous modifications, and moreover, by continuity,  $F_1$  and  $F_2$  are indistinguishable from these modifications.

We turn to the proof of (A.1). For an arbitrary fixed  $\gamma \in \Gamma$ , define the time-changed ‘bridge’ process  $X_\gamma$  by

$$X_\gamma(u) := M_\gamma(u) - \frac{V_\gamma(u)}{V_\gamma(1)} M_\gamma(1), \quad u \in [0, 1].$$

Then  $X_\gamma$  and  $M_\gamma(1)$  are independent, for they are jointly Gaussian with covariance function

$$\text{Cov}(X_\gamma(u), M_\gamma(1)) = V_\gamma(u) - \frac{V_\gamma(u)}{V_\gamma(1)} V_\gamma(1) = 0, \quad u \in [0, 1].$$

In terms of  $X_\gamma$  and  $M_\gamma(1)$ , we find

$$\tau_{\gamma 1} = \frac{1}{2} \frac{M_\gamma(1)^2 - V_\gamma(1)}{\int_0^1 M_\gamma^2(u) du} = \frac{1}{2} \frac{M_\gamma(1)^2 - V_\gamma(1)}{\int_0^1 (X_\gamma(u) + M_\gamma(1)q_\gamma(u))^2 du}$$

and

$$\tau_{\gamma 2} = \frac{1}{2} \frac{M_\gamma(1)^2 - V_\gamma(1)}{\sqrt{V_\gamma(1) \int_0^1 (X_\gamma(u) + M_\gamma(1)q_\gamma(u))^2 du}},$$

for  $q_\gamma(u) := V_\gamma(u)/V_\gamma(1)$ . The equality

$$P(\tau_{\gamma i} = x) = E[P(\tau_{\gamma i} = x | M_\gamma(1))] = 0$$

will hold for  $i = 1, 2$  and any  $x \in \mathbb{R}$  iff

$$P(\tau_{\gamma i} = x | M_\gamma(1)) = 0 \text{ a.s.}$$

for  $i = 1, 2$  and any  $x \in \mathbb{R}$ . In its turn, using the independence of  $X_\gamma(u)$  and  $M_\gamma(1)$ , the latter will hold if

$$P\left(\frac{1}{2} \frac{\alpha^2 - V_\gamma(1)}{\int_0^1 (X_\gamma(1) + \alpha q_\gamma(u))^2 du} = x\right) = 0,$$

$$P\left(\frac{1}{2} \frac{\alpha^2 - V_\gamma(1)}{\sqrt{V_\gamma(1) \int_0^1 (X_\gamma(u) + \alpha q_\gamma(u))^2 du}} = x\right) = 0$$

hold for all  $x \in \mathbb{R}$  and  $\alpha \neq \pm\sqrt{V_\gamma(1)}$  (because  $P(M_\gamma^2(1) = V_\gamma(1)) = 0$ ), which in its turn will hold if

$$P\left(\int_0^1 (X_\gamma(u) + \alpha q_\gamma(u))^2 du = x\right) = 0$$

for any  $\alpha, x \in \mathbb{R}$ . Since  $X_\gamma$  is a zero-mean Gaussian process with a continuous covariance and  $q_\gamma$  is square integrable, the equality in the previous display indeed holds, by Rao and Swift (2006, pp. 472–473).  $\square$

## A.2 PROOFS

PROOF OF LEMMA 1. We follow the approach of the proof of Lemma 1 and other intermediate results in Cavaliere and Taylor (2009). First, defining  $e_t = z_t^2 - 1$ ,

$$\sup_{u \in [0,1]} |U_n(u) - V_n(u)| = \sup_{u \in [0,1]} \left| n^{-1} \sum_{t=1}^{\lfloor nu \rfloor} \sigma_t^2 e_t \right| \xrightarrow{p} 0$$

by Theorem A.1 of Cavaliere and Taylor (2009), since  $\{e_t, \mathcal{F}_t\}_{t \geq 1}$  is an mds by Assumption 1 and  $\sigma_{\lfloor n \cdot \rfloor + 1}^2 = \sigma_n^2(\cdot) \xrightarrow{w} \sigma^2(\cdot)$  by Assumption 2 and the CMT; this proves (8), because convergence in the sup norm implies convergence in the Skorokhod metric, i.e., in  $\mathcal{D}[0, 1]$ . Next, we apply Theorem 2.1 of Hansen (1992) to

$$M_n(\cdot) = \int_0^\cdot \sigma_n(u) dB_{z,n}(u),$$

noting that Assumption 1 implies  $\sup_{n \geq 1} n^{-1} \sum_{t=1}^n E(z_t^2) = 1$ , so that using Assumption 2, we have

$$(\sigma_n(\cdot), B_{z,n}(\cdot), M_n(\cdot)) \xrightarrow{w} (\sigma(\cdot), B_z(\cdot), M(\cdot)).$$

The CMT together with (8) then implies (7), because

$$\int_0^u \sigma_n^2(s) ds = \frac{1}{n} \sum_{t=1}^{\lfloor nu \rfloor} \sigma_t^2 + \sigma_{\lfloor nu \rfloor + 1}^2 (u - \lfloor nu \rfloor n^{-1}), \quad u \in [0, 1],$$

so that  $U_n(\cdot) = V_n(\cdot) + o_p(1) = \int_0^\cdot \sigma_n^2(s) ds + o_p(1)$ , i.e.,  $U_n(\cdot)$  is a continuous functional of  $\sigma_n(\cdot)$  plus an asymptotically negligible term.  $\square$

PROOF OF THEOREM 1. The idea of the proof is to construct on a special probability space random elements distributed like  $(\sigma_n, M_n, U_n, M_n^*, U_n^*)$  and such that on this probability space the convergence asserted in Theorem 1 holds weakly a.s.; on a general probability space it will then hold  $\xrightarrow{w}$ . Throughout, we use repeatedly the fact that for independent random elements  $\xi$  and  $\eta$  and for a measurable real  $\phi$  such that  $E(|\phi(\xi, \eta)|) < \infty$ , it holds that  $E(\phi(\xi, \eta)|\eta) = E(\phi(\xi, v))|_{v=\eta}$  a.s., with  $E(\phi(\xi, v))$  defining a function of a non-random  $v$ ; see Dudley (2004, p. 341).

By Assumption 3,  $\psi_{nt}$  are  $\mathcal{G}_{n0}$ -measurable and hence are measurable functions of  $\sigma_n$  that we denote, with a slight abuse of notation, by  $\psi_{nt}(\sigma_n)$ . Let

$$e_{nm}(\gamma) := E\left(v_{nt}^2 \psi_{nt}^2(\gamma) \mathbb{I}_{\{|v_{nt} \psi_{nt}(\gamma)| > \sqrt{n}/m\}}\right),$$

for  $m \in \mathbb{N}$  and a generic non-random  $\gamma$ ; then  $e_{nm}(\sigma_n)$  is a version of the conditional expectation  $E\left(z_t^2 \mathbb{I}_{\{|z_t| > \sqrt{n}/m\}} | \sigma_n\right)$  because  $\{v_{nt}\}_{t=1}^n$  and  $\sigma_n$  are independent. Define  $B_{v,n}(\cdot) := n^{-1/2} \sum_{t=1}^{\lfloor n \cdot \rfloor} v_{nt}$ . We apply Theorem A.1 with  $\xi_n = (\sigma_n, B_{v,n})$ ,  $\xi = (\sigma, B_z)$ ,

$$f_n(\xi_n) = (\sigma_n, Q_{\psi,n}, Q_{z,n}, \mathcal{L}_n, L_n) \text{ and } f(\xi) = (\sigma, Q, Q, 0^\infty, 0^\infty),$$

where  $Q_{\psi,n}(\cdot) = n^{-1} \sum_{t=1}^{\lfloor n \cdot \rfloor} \psi_{nt}^2$ ,  $Q_{z,n}(\cdot) = n^{-1} \sum_{t=1}^{\lfloor n \cdot \rfloor} z_t^2$ ,  $\mathcal{L}_n = \{n^{-1} \sum_{t=1}^n e_{nm}(\sigma_n)\}_{m \in \mathbb{N}} \in \mathbb{R}^\infty$ ,  $L_n = \left\{n^{-1} \sum_{t=1}^n z_t^2 \mathbb{I}_{\{|z_t| > \sqrt{n}/m\}}\right\}_{m \in \mathbb{N}} \in \mathbb{R}^\infty$ ,  $Q(u) = u, u \in [0, 1]$ , and  $0^\infty$  is the zero sequence in  $\mathbb{R}^\infty$ , the Frechet space. The domain of  $f_n$  and  $f$  is the Borel space  $\mathcal{D}_2[0, 1]$  with the Skorokhod metric and the induced Borel  $\sigma$ -algebra, and the codomain is the Polish space  $\mathcal{D}_3[0, 1] \times \mathbb{R}^\infty \times \mathbb{R}^\infty$  with the product of the Skorokhod and the Frechet metric. The assumptions imply  $(Q_{\psi,n}, Q_{z,n}) \xrightarrow{P} (Q, Q)$ , because  $(Q_{\psi,n} - Q, Q_{z,n} - Q)$  is the partial sum process of  $n^{-1}(\psi_{nt}^2 - 1, z_t^2 - 1)$ , which is an mda with respect to  $\mathcal{F}_t$  since  $E(\psi_{nt}^2 | \mathcal{F}_{t-1}) = E(z_t^2 | \mathcal{F}_{t-1}) = 1$  by the tower property; this partial sum converges to the zero function in probability by the corollary to Theorem 3.3 of Hansen (1992). Noting that  $L_n \xrightarrow{P} 0^\infty$  follows from the corresponding result for  $\mathcal{L}_n = E(L_n | \mathcal{G}_{n0})$ , applying Markov's inequality, the assumptions therefore imply  $f_n(\xi_n) \xrightarrow{w} f(\xi)$ .

Theorem A.1 then implies the existence of  $\tilde{\xi}_n = (\tilde{\sigma}_n, \tilde{B}_{v,n}) \stackrel{d}{=} (\sigma_n, B_{v,n})$  and  $\tilde{\xi} = (\tilde{\sigma}, \tilde{B}_z) \stackrel{d}{=} (\sigma, B_z)$ , defined on a single probability space and such that

$$(\tilde{\sigma}_n, \tilde{Q}_{\psi,n}, \tilde{Q}_{z,n}, \tilde{\mathcal{L}}_n, \tilde{L}_n) := f_n(\tilde{\xi}_n) \xrightarrow{a.s.} f(\tilde{\xi}) = (\tilde{\sigma}, Q, Q, 0^\infty, 0^\infty). \quad (\text{A.2})$$

Finally, we complete the set up by introducing a product extension of the previous probability space where a sequence  $\{\tilde{w}_t^*\} \stackrel{d}{=} \{w_t^*\}$  and a standard Brownian motion  $\tilde{B}_z^*$  are defined and are independent of  $\{(\tilde{\sigma}_n, \tilde{B}_{v,n})\}_{n \geq 1}$  and  $(\tilde{\sigma}, \tilde{B}_z)$ .

As  $\tilde{B}_{v,n}$  and  $\tilde{\sigma}_n$  are independent (because  $B_{v,n}$  and  $\sigma_n$  are), it holds for any integrable random variable  $h(\tilde{\sigma}_n, \tilde{B}_{v,n})$  that  $E(h(\tilde{\sigma}_n, \tilde{B}_{v,n}) | \tilde{\sigma}_n) = E(h(\gamma, \tilde{B}_{v,n}) | \gamma = \tilde{\sigma}_n)$ . A similar equality holds for the independent  $\tilde{B}_z$  and  $\tilde{\sigma}$ . Therefore, to prove any convergence of the form

$$E\left(h_n(\tilde{\sigma}_n, \tilde{B}_{v,n}) | \tilde{\sigma}_n\right) \xrightarrow{a.s.} E\left(h(\tilde{\sigma}, \tilde{B}_z) | \sigma\right), \quad (\text{A.3})$$

it is sufficient to prove that  $E(h_n(\gamma_n, \tilde{B}_{v,n})) \rightarrow E(h(\gamma, \tilde{B}_z))$  for all deterministic sequences  $\{\gamma_n\}_{n \geq 1}$  in some set  $\Gamma \subset \mathcal{D}_\infty[0, 1]$  such that  $P(\{\tilde{\sigma}_n\}_{n \geq 1} \in \Gamma) = 1$ . We now choose and fix  $\Gamma$ . Consider all the outcomes  $\tilde{\omega}$  such that convergence (A.2) holds; the set of such outcomes  $\tilde{\omega}$  has probability 1. Define  $\Gamma \subset \mathcal{D}_\infty[0, 1]$  as the set of sequences  $\{\tilde{\sigma}_n(\cdot, \tilde{\omega})\}_{n \geq 1}$  corresponding to such  $\tilde{\omega}$ , then  $P(\{\tilde{\sigma}_n\}_{n \geq 1} \in \Gamma) = 1$  as required.

As noted in Remark 4.4, we may recover  $(M_n, U_n)$  (and hence the original data  $D_n$ ) from  $(\sigma_n, B_{v,n})$  as some measurable transformation, say  $m_n(\sigma_n, B_{v,n})$ . Define accordingly  $(\tilde{M}_n, \tilde{U}_n) := m_n(\tilde{\sigma}_n, \tilde{B}_{v,n})$  (and analogously  $\tilde{D}_n$ ). With  $\tilde{z}_{nt} := \tilde{\psi}_{nt} \tilde{v}_{nt}$ , where  $\tilde{\psi}_{nt} = \psi_{nt}(\tilde{\sigma}_n)$  and

$$\tilde{v}_{nt} := n^{1/2} \left( \tilde{B}_{v,n}(t/n) - \tilde{B}_{v,n}((t-1)/n) \right),$$

define also the process  $\tilde{B}_{z,n}(\cdot) := n^{-1/2} \sum_{t=1}^{\lfloor n \cdot \rfloor} \tilde{z}_{nt} =: m_{z,n}(\tilde{\sigma}_n, \tilde{B}_{v,n})$ , such that

$$(\tilde{\sigma}_n, \tilde{B}_{z,n}, \tilde{M}_n, \tilde{U}_n) \stackrel{d}{=} (\sigma_n, B_{z,n}, M_n, U_n).$$

We proceed to the convergence of  $(\tilde{M}_n, \tilde{U}_n)$  conditional on  $\tilde{\sigma}_n$  and prove that

$$E\left(g(\tilde{B}_{z,n}, \tilde{M}_n, \tilde{U}_n) \middle| \tilde{\sigma}_n\right) \xrightarrow{a.s.} E\left(g(\tilde{B}_z, \tilde{M}, \tilde{V}) \middle| \tilde{\sigma}\right) \quad (\text{A.4})$$

for continuous bounded real  $g$  of matching domain; this convergence is of the form (A.3) with  $h_n = g \circ (m_{z,n}, m_n)$ . In so doing, for any random element  $Z = \phi(\tilde{\sigma}_n, \tilde{B}_{v,n})$  we write  $Z(\gamma_n)$  for  $\phi(\gamma_n, \tilde{B}_{v,n})$ ; e.g.,  $\tilde{B}_{z,n}(\gamma_n) = m_{z,n}(\gamma_n, \tilde{B}_{v,n})$ . By the discussion in the previous paragraph, (A.4) will follow from the standard weak convergence of  $(\tilde{B}_{z,n}(\gamma_n), \tilde{M}_n(\gamma_n), \tilde{U}_n(\gamma_n))$ , for all  $\{\gamma_n\}_{n \geq 1} \in \Gamma$ , that we establish next.

For  $\{\tilde{\sigma}_n\}_{n \in \mathbb{N}}$  replaced by a fixed  $\{\gamma_n\}_{n \geq 1} \in \Gamma$ ,  $\tilde{z}_{nt}(\gamma_n) = \psi_{nt}(\gamma_n)\tilde{v}_{nt}$  is an mda satisfying the conditions of Brown (1971)'s functional central limit theorem. First,  $E(\psi_{nt}(\gamma_n)\tilde{v}_{nt} | \{\tilde{v}_{ni}\}_{i=1}^{t-1}) = \psi_{nt}(\gamma_n)E(\tilde{v}_{nt} | \{\tilde{v}_{ni}\}_{i=1}^{t-1}) = 0$  because the mda property of  $\tilde{v}_{nt}$  is inherited from the original probability space as  $\{\tilde{v}_{ni}\}_{i=1}^n \stackrel{d}{=} \{v_{ni}\}_{i=1}^n$ . Second,  $n^{-1} \sum_{t=1}^{\lfloor n \rfloor} E(\psi_{nt}^2(\gamma_n)\tilde{v}_{nt}^2 | \{\tilde{v}_{ni}\}_{i=1}^{t-1}) = n^{-1} \sum_{t=1}^{\lfloor n \rfloor} \psi_{nt}^2(\gamma_n) = \tilde{Q}_{\psi,n}(\cdot, \gamma_n) \rightarrow Q(\cdot)$ , where the first equality is again inherited from the original probability space, and the convergence by the definition of  $\Gamma$ . Third, as  $\tilde{\mathcal{L}}_n(\gamma_n) \rightarrow 0^\infty$  again by the choice of  $\Gamma$ , it holds that  $n^{-1} \sum_{t=1}^n e_{nm}(\gamma_n) \rightarrow 0$  for all  $m \in \mathbb{N}$ , which is equivalent to

$$n^{-1} \sum_{t=1}^n E\left(\tilde{z}_{nt}^2(\gamma_n) \mathbb{I}_{\{|\tilde{z}_{nt}(\gamma_n)| > \sqrt{n}/m\}}\right) \rightarrow 0, \quad m \in \mathbb{N},$$

by the definition of  $e_{nm}$  and implies the Lindeberg condition in its usual form

$$n^{-1} \sum_{t=1}^n E\left(\tilde{z}_{nt}^2(\gamma_n) \mathbb{I}_{\{|\tilde{z}_{nt}(\gamma_n)| > \sqrt{n}\epsilon\}}\right) \rightarrow 0$$

for all  $\epsilon > 0$ . Therefore,

$$\tilde{B}_{z,n}(\gamma_n) \xrightarrow{w} \tilde{B}_z,$$

in the sense that  $E(g(\tilde{B}_{z,n}(\gamma_n))) \rightarrow E(g(\tilde{B}_z))$  for continuous bounded real  $g$  with matching domain. For the same fixed  $\gamma_n$ , this in turn implies that

$$\tilde{M}_n(\cdot, \gamma_n) = \int_0^\cdot \gamma_n(u) d\tilde{B}_{z,n}(u, \gamma_n) \xrightarrow{w} \int_0^\cdot \gamma(u) d\tilde{B}_z(u),$$

where  $\gamma = \lim \gamma_n$  exists by the choice of  $\gamma_n$ . More precisely, by Theorem 2.1 of Hansen (1995), as  $\sup_{n \geq 1} \sum_{t=1}^n E(\tilde{z}_{nt}^2(\gamma_n)) = \sup_{n \geq 1} \tilde{Q}_{\psi,n}(1, \gamma_n) < \infty$ , the previous convergence holds jointly with that of  $\tilde{B}_{z,n}$ , such that  $E(g(\tilde{B}_{z,n}(\gamma_n), \tilde{M}_n(\cdot, \gamma_n))) \rightarrow E(g(\tilde{B}_z, \int_0^\cdot \gamma d\tilde{B}_z))$  for continuous bounded real  $g$ . Furthermore, using

$$\begin{aligned} \tilde{U}_n(\cdot) &= n^{-1} \sum_{t=1}^{\lfloor n \rfloor} \tilde{\sigma}_t^2 \tilde{\psi}_{nt}^2 + n^{-1} \sum_{t=1}^{\lfloor n \rfloor} \tilde{\sigma}_t^2 \left( \tilde{z}_{nt}^2 - \tilde{\psi}_{nt}^2 \right) \\ &= \int_0^\cdot \tilde{\sigma}_n^2(u) d\tilde{Q}_{\psi,n}(u) + n^{-1} \sum_{t=1}^{\lfloor n \rfloor} \tilde{\sigma}_t^2 \tilde{e}_{nt}, \end{aligned}$$

it follows that  $\tilde{U}_n(\cdot, \gamma_n) \xrightarrow{p} \int_0^\cdot \gamma^2(u) du$  by Theorem A.1 of Cavaliere and Taylor (2009), since  $\tilde{z}_{nt}^2(\gamma_n) - \tilde{\psi}_{nt}^2(\gamma_n)$  is an mda. As convergence in probability to a constant is joint with any weak

convergence of random elements defined on the same probability space, it follows that

$$E \left[ g(\tilde{B}_{z,n}(\gamma_n), \tilde{M}_n(\cdot, \gamma_n), \tilde{U}_n(\cdot, \gamma_n)) \right] \rightarrow E \left[ g \left( \tilde{B}_z, \int_0^\cdot \gamma d\tilde{B}_z, \int_0^\cdot \gamma^2 \right) \right]$$

for continuous bounded real  $g$ . Since  $P(\Gamma) = 1$ ,  $(\tilde{B}_z, \int_0^\cdot \gamma d\tilde{B}_z, \int_0^\cdot \gamma^2)|_{\gamma=\tilde{\sigma}} = (\tilde{B}_z, \tilde{M}, \tilde{V})$  and  $\tilde{B}_z$  is independent of  $\tilde{\sigma}$ , we can conclude that (A.4) holds.

We turn to the bootstrap processes. Define

$$\tilde{B}_{z,n}^*(\cdot) := n^{-1/2} \sum_{t=1}^{\lfloor n \rfloor} \tilde{z}_{nt} \tilde{w}_t^*, \quad \tilde{M}_n^*(\cdot) := n^{-1/2} \sum_{t=1}^{\lfloor n \rfloor} \tilde{\sigma}_t \tilde{z}_{nt} \tilde{w}_t^*, \quad \tilde{U}_n^*(\cdot) := n^{-1} \sum_{t=1}^{\lfloor n \rfloor} \tilde{\sigma}_t^2 \tilde{z}_{nt}^2 \tilde{w}_t^{*2}.$$

Here we show that

$$E \left( g(\tilde{B}_{z,n}^*, \tilde{M}_n^*, \tilde{U}_n^*) \middle| \tilde{\sigma}_n, \tilde{B}_{v,n} \right) \xrightarrow{a.s.} E \left( g(\tilde{B}_z^*, \tilde{M}^*, \tilde{V}) \middle| \tilde{\sigma} \right)$$

for continuous bounded real  $g$ , where  $\tilde{B}_z^*$  is a standard Brownian motion independent of  $(\tilde{\sigma}, \tilde{B}_z)$ , and  $\tilde{M}^*(\cdot) := \int_0^\cdot \tilde{\sigma} d\tilde{B}_z^*$ . Given that  $\{\tilde{w}_t^*\}$  and  $(\tilde{\sigma}, \tilde{B}_z)$  are independent, as in the proof of (A.4), we could proceed by fixing  $\{(\gamma_n, b_n)\}_{n \geq 1} \in \Gamma B$ , where  $\Gamma B$  is an appropriate set with  $P((\tilde{\sigma}_n, \tilde{B}_{v,n})_{n \geq 1} \in \Gamma B) = 1$ , and then discuss the standard weak convergence of  $(\tilde{B}_{z,n}^*, \tilde{M}_n^*, \tilde{U}_n^*)$  as a transformation of  $(\gamma_n, b_n, \{\tilde{w}_t^*\})$  instead of  $(\tilde{\sigma}, \tilde{B}_z, \{\tilde{w}_t^*\})$ . Since now  $(\tilde{\sigma}_n, \tilde{B}_{v,n})$  and  $\{\tilde{w}_t^*\}$  are defined on a product space, we implement this equivalently by fixing outcomes  $\tilde{\omega}$  in the component space of  $(\tilde{\sigma}_n, \tilde{B}_{v,n})$  and letting the outcome in the component space of  $\{\tilde{w}_t^*\}$  be the only source of randomness. In what follows, fix an  $\tilde{\omega}$  in a probability-one set where convergence (A.2) holds. Then

$$n^{-1/2} \sum_{t=1}^{\lfloor n \rfloor} \tilde{z}_{nt}(\tilde{\omega}) \tilde{w}_t^* \xrightarrow{w} B_z^*(\cdot),$$

because  $n^{-1} \sum_{t=1}^{\lfloor n \rfloor} \tilde{z}_{nt}^2(\tilde{\omega}) = Q_{z,n}(\cdot, \tilde{\omega}) \rightarrow Q(\cdot)$  and  $L_n(\tilde{\omega}) \rightarrow 0^\infty$  by the choice of  $\tilde{\omega}$ , where

$$L_n(\tilde{\omega}) = \left\{ n^{-1} \sum_{t=1}^{\lfloor n \rfloor} \tilde{z}_{nt}^2(\tilde{\omega}) \mathbb{I}(|\tilde{z}_{nt}(\tilde{\omega})| > \sqrt{n}/m) \right\}_{m \in \mathbb{N}}.$$

It follows that  $\tilde{M}_n^*(\cdot, \tilde{\omega}) = n^{-1/2} \sum_{t=1}^{\lfloor n \rfloor} \tilde{\sigma}_t(\tilde{\omega}) \tilde{z}_{nt}(\tilde{\omega}) \tilde{w}_t^* \xrightarrow{w} \int_0^\cdot \tilde{\sigma}(\tilde{\omega}) d\tilde{B}_z^*$ . Further,

$$\begin{aligned} \tilde{U}_n^*(\cdot, \tilde{\omega}) &= n^{-1} \sum_{t=1}^{\lfloor n \rfloor} \tilde{\sigma}_t^2(\tilde{\omega}) \tilde{z}_{nt}^2(\tilde{\omega}) \tilde{w}_t^{*2} \\ &= \tilde{U}_n(\cdot) + n^{-1} \sum_{t=1}^{\lfloor n \rfloor} \tilde{\sigma}_t^2(\tilde{\omega}) \tilde{z}_{nt}^2(\tilde{\omega}) (\tilde{w}_t^{*2} - 1) \xrightarrow{p} \tilde{V}(\cdot, \tilde{\omega}), \end{aligned}$$

using Theorem A.1 of Cavaliere and Taylor (2009). Since  $\tilde{V}(\cdot, \tilde{\omega})$  is non-random, the last two convergences are joint:

$$E \left[ g \left( \tilde{M}_n^*(\cdot, \tilde{\omega}), \tilde{U}_n^*(\cdot, \tilde{\omega}) \right) \right] \rightarrow E \left[ g \left( \tilde{M}^*(\cdot, \tilde{\omega}), \tilde{V}(\cdot, \tilde{\omega}) \right) \right]$$

for continuous and bounded real  $g$ . This implies, by the product structure of the probability space and the probability-one set of eligible outcomes  $\tilde{\omega}$ , that

$$E \left( g(\tilde{M}_n^*, \tilde{U}_n^*) | \tilde{\sigma}_n, \tilde{B}_{v,n} \right) \xrightarrow{a.s.} E \left( g(\tilde{M}^*, \tilde{V}) | \tilde{\sigma} \right),$$

and eventually, as  $(\tilde{M}^*, \tilde{V}, \tilde{\sigma}) \stackrel{d}{=} (\tilde{M}, \tilde{V}, \tilde{\sigma})$ , that

$$E \left( g(\tilde{M}_n^*, \tilde{U}_n^*) | \tilde{\sigma}_n, \tilde{B}_{v,n} \right) \xrightarrow{a.s.} E \left( g(\tilde{M}, \tilde{V}) | \tilde{\sigma} \right).$$

Notice that conditioning on  $\tilde{\sigma}_n, \tilde{B}_{v,n}$  can be replaced by conditioning on  $\tilde{D}_n$  because  $(\tilde{M}_n^*, \tilde{U}_n^*)$  is a measurable function of  $\tilde{D}_n$  and  $\{\tilde{w}_t^*\}$ .

We can conclude from (A.4) and this result that

$$\left( E \left[ h(\tilde{M}_n, \tilde{U}_n) | \tilde{\sigma}_n \right], E \left[ g(\tilde{M}_n^*, \tilde{U}_n^*) | \tilde{D}_n \right] \right) \xrightarrow{a.s.} \left( E \left[ h(\tilde{M}, \tilde{V}) | \tilde{\sigma} \right], E \left[ g(\tilde{M}, \tilde{V}) | \tilde{\sigma} \right] \right)$$

for all continuous and bounded real  $h, g$ , whereas on a general probability space

$$(E[h(M_n, U_n) | \sigma_n], E[g(M_n^*, U_n^*) | D_n]) \xrightarrow{w} (E[h(M, V) | \sigma], E[g(M, V) | \sigma]), \quad (\text{A.5})$$

because  $(\tilde{\sigma}_n, \tilde{M}_n, \tilde{U}_n, \tilde{D}_n, \tilde{M}_n^*, \tilde{U}_n^*) \stackrel{d}{=} (\sigma_n, M_n, U_n, D_n, M_n^*, U_n^*)$ . This is precisely the definition of the joint  $\xrightarrow{w}$  convergence in the theorem.  $\square$

PROOF OF COROLLARY 1. From (A.5) with  $h = g = \tau$ , if the random cdf  $P(\tau(M, V) \leq \cdot | \sigma)$  a.s. has continuous sample paths, conditional validity of the bootstrap as in Corollary 1 follows from Corollary 3.2 of Cavaliere and Georgiev (2020).  $\square$

PROOF OF LEMMA 1. For any  $K \in \mathbb{R}$ , consider the continuous function  $g_K : \mathbb{R} \rightarrow [0, 1]$  defined by  $g_K(x) = \mathbb{I}_{(-\infty, K]}(x) + (K + 1 - x)\mathbb{I}_{(K, K+1]}$ . Then  $\mathbb{I}_{(-\infty, K]} \leq g_K \leq \mathbb{I}_{(-\infty, K+1]}$  and the convergence  $\tau_n^* \xrightarrow{w} \tau^* | \sigma$  implies that

$$F_n^*(K) \leq E^*(g_K(\tau_n^*)) \xrightarrow{w} E(g_K(\tau) | \sigma) \leq F^*(K + 1),$$

where  $F^*(K + 1) = P(\tau^* \leq K + 1 | \sigma)$ . Therefore, for all  $q \in (0, 1)$ ,

$$\liminf_{n \rightarrow \infty} P(F_n^*(K) \leq q) \geq P(F^*(K + 1) \leq q).$$

As a result,

$$\begin{aligned} \liminf_{n \rightarrow \infty} P(F_n^*(\tau_n) \leq q) &\geq \liminf_{n \rightarrow \infty} P(F_n^*(\tau_n) \leq q, \tau_n \leq K) \\ &\geq \liminf_{n \rightarrow \infty} P(F_n^*(K) \leq q, \tau_n \leq K) \\ &\geq \liminf_{n \rightarrow \infty} P(F_n^*(K) \leq q) - \lim_{n \rightarrow \infty} P(\tau_n > K) \\ &\geq P(F^*(K + 1) \leq q), \end{aligned}$$

since  $\tau_n \xrightarrow{P} -\infty$  means that  $\lim_{n \rightarrow \infty} P(\tau_n > K) = 0$  for all  $K \in \mathbb{R}$ . By Markov's inequality,

$$P(F^*(K + 1) \leq q) \geq 1 - q^{-1} E(F^*(K + 1)) = 1 - q^{-1} P(\tau^* \leq K + 1),$$

and the proof is completed by letting  $K \rightarrow -\infty$ .  $\square$

PROOF OF EQ. (23). Notice that

$$\hat{U}_n(\cdot) = n^{-1} \sum_{t=1}^{\lfloor n \cdot \rfloor} \left( \sum_{i=0}^{t-1} \psi_i \varepsilon_{t-i} \right)^2$$

$$\begin{aligned}
&= n^{-1} \sum_{t=1}^{\lfloor n \cdot \rfloor} \sum_{i=0}^{t-1} \psi_i^2 \varepsilon_{t-i}^2 + 2n^{-1} \sum_{t=1}^{\lfloor n \cdot \rfloor} \sum_{i=0}^{t-1} \sum_{j=0}^{i-1} \psi_i \psi_j \varepsilon_{t-i} \varepsilon_{t-j} \\
&=: a_{1n}(\cdot) + a_{2n}(\cdot),
\end{aligned}$$

with  $a_{1n}(\cdot)$  and  $a_{2n}(\cdot)$  implicitly defined. First,  $a_{2n}(\cdot) = o_p(1)$  uniformly in  $\cdot \in [0, 1]$ , similarly to Lemma A.7 in Cavaliere *et al.* (2010a). Second,

$$a_{1n}(\cdot) = n^{-1} \sum_{t=1}^{\lfloor n \cdot \rfloor} \varepsilon_t^2 \left( \sum_{i=0}^{\lfloor n \cdot \rfloor - t} \psi_i^2 \right) = \left( \sum_{i=0}^{\infty} \psi_i^2 \right) U_n(\cdot) + b_n(\cdot),$$

with

$$b_n(\cdot) := n^{-1} \sum_{t=1}^{\lfloor n \cdot \rfloor} \varepsilon_t^2 \left( \sum_{i=\lfloor n \cdot \rfloor - t + 1}^{\infty} \psi_i^2 \right).$$

Since the  $\psi_i$ 's are exponentially decaying, there exist constants  $C$  and  $\rho \in (0, 1)$  such that  $\sum_{i=\lfloor n \cdot \rfloor - t + 1}^{\infty} \psi_i^2 \leq C\rho^{\lfloor n \cdot \rfloor - t + 1}$ . Using the facts that  $\max_{t=1, \dots, n} \sigma_t^2 = O_p(1)$  by Assumption 2 and  $E(z_t^2) = 1$  by Assumption 1, it holds that

$$\begin{aligned}
\sup_{u \in [0, 1]} b_n(u) &\leq Cn^{-1} \sup_{u \in [0, 1]} \sum_{t=1}^{\lfloor nu \rfloor} \sigma_t^2 z_t^2 \rho^{\lfloor n \cdot \rfloor - t + 1} \\
&\leq C \left( \max_{t=1, \dots, n} \sigma_t^2 \right) \left( n^{-1} \max_{t=1, \dots, n} z_t^2 \right) \sup_{u \in [0, 1]} \left( \sum_{t=1}^{\lfloor n \cdot \rfloor} \rho^{\lfloor n \cdot \rfloor - t + 1} \right) \\
&= O_p(1) o_p(1) \sum_{t=1}^n \rho^t = o_p(1).
\end{aligned}$$

Hence,  $\hat{U}_n(\cdot) = (\sum_{i=0}^{\infty} \psi_i^2) U_n(\cdot) + o_p(1)$ . □

## REFERENCES

- Brown, B. M. (1971), “Martingale Central Limit Theorems”, *Annals of Mathematical Statistics* 42, 59–66.
- Cavaliere, G. and I. Georgiev (2020), “Inference Under Random Limit Bootstrap Measures”, *Econometrica* 88, 2547–2574.
- Cavaliere, G., A. Rahbek and A. M. R. Taylor (2010a), “Testing for Co-Integration in Vector Autoregressions with Non-Stationary Volatility”, *Journal of Econometrics* 158, 7–24.
- Cavaliere, G. and A. M. R. Taylor (2009), “Heteroskedastic Time Series with a Unit Root”, *Econometric Theory* 25, 1228–1276.
- Dudley, R. M. (2004), *Real Analysis and Probability*. Cambridge: Cambridge University Press.
- Hansen, B. E. (1992), “Convergence to Stochastic Integrals for Dependent Heterogeneous Processes”, *Econometric Theory* 8, 489–500.
- Hansen, B. E. (1995), “Regression with Nonstationary Volatility”, *Econometrica* 63, 1113–1132.
- Kallenberg, O. (1997), *Foundations of Modern Probability*. New York: Springer.
- Rao, M. M. and R. J. Swift (2006). *Probability Theory with Applications*. New York: Springer.
